# Supplementary material for: Bonding Description of the Harpoon Mechanism
Source: arXiv:1510.07687 source file (2015-11-11)
Supplement: Supplementary file 1 [file SuppInfo.pdf]

# Bonding Description of the Harpoon Mechanism

## Supporting Information

M. Rodríguez-Mayorga, E. Ramos-Cordoba, P. Salvador, M. Solà and E. Matito

November 9, 2015

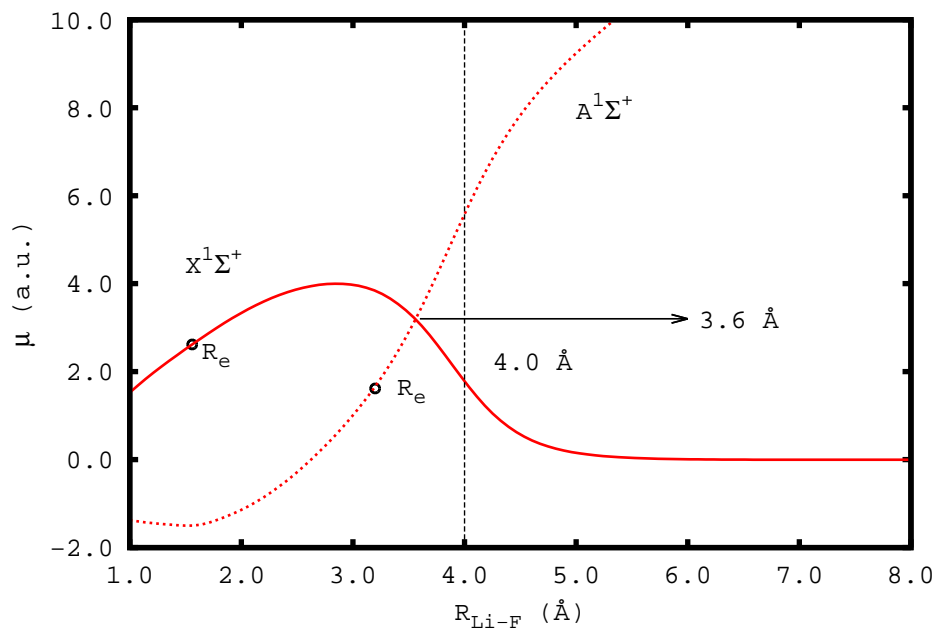

Figure S1: Dipole moment (in a.u.) along the internuclear axis for the  $X^1\Sigma^+$  and the  $A^1\Sigma^+$  states of LiF as function of the interatomic distance.

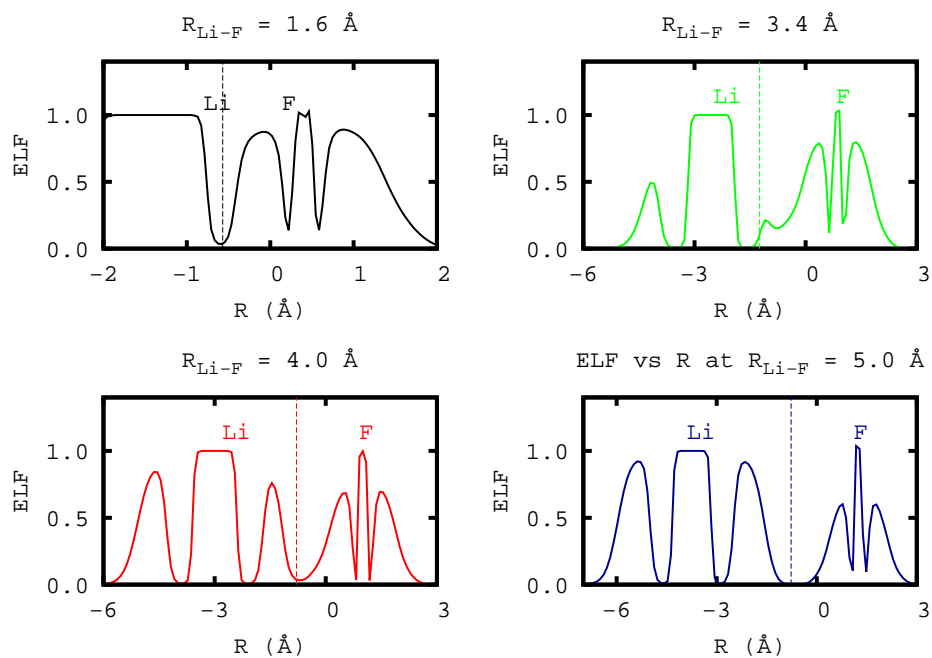

Figure S2: The ELF profile of the  $A^1\Sigma^+$  state of LiF along the internuclear axis for several values of the interatomic distance. The zero is located at the center of mass and the vertical dashed line indicates the bond critical point.

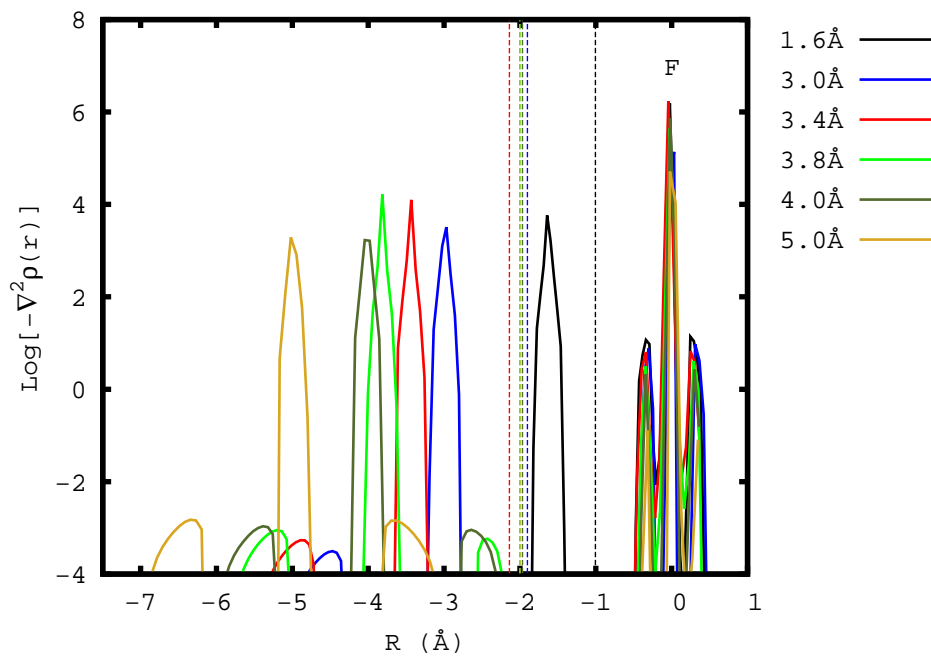

Figure S3: The negative values of the Laplacian of the electron density of LiF's  $X^1\Sigma^+$  state along the internuclear axis as function of the interatomic distance for several interatomic distances. All molecules locate Li atom in the z-axis at zero for comparison. The vertical dashed line indicates the bond critical point. Laplacian units are a.u.

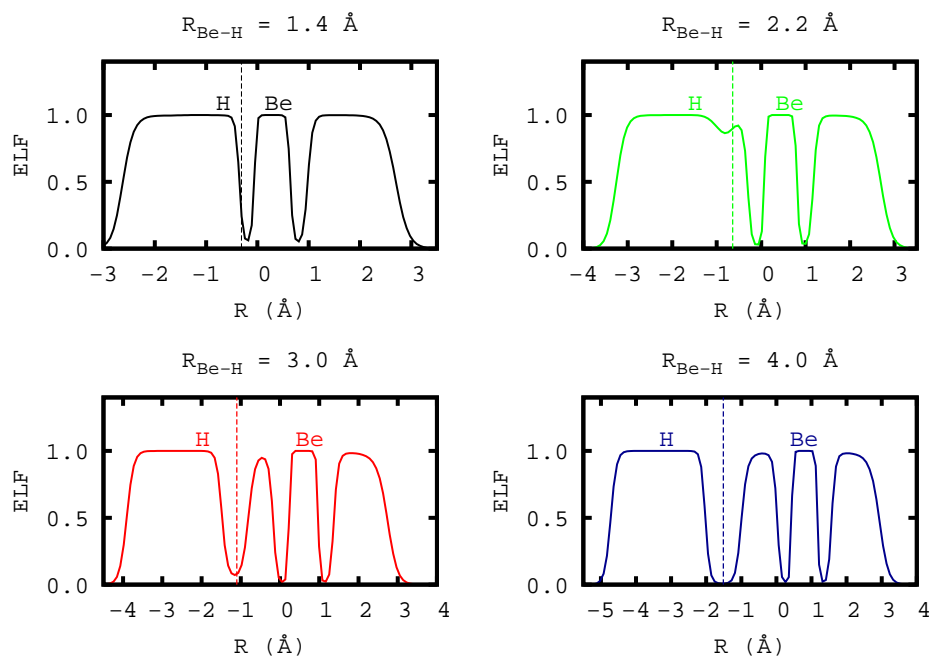

Figure S4: The ELF profile of the  $X^2\Sigma^+$  state of BeH along the internuclear axis for several values of the interatomic distance. The zero is located at the center of mass and the vertical dashed line indicates the bond critical point.

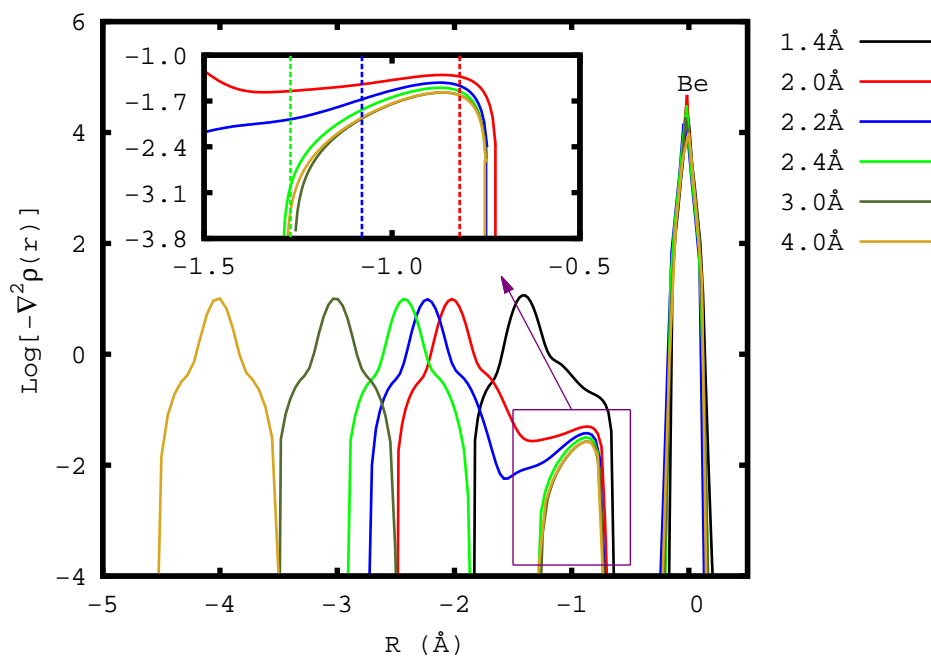

Figure S5: The negative values of the Laplacian of the electron density of BeH along the inter-nuclear axis for several interatomic distances. All molecules locate Be atom in the z-axis at zero for comparison. The vertical dashed line indicates the bond critical point. Laplacian units are a.u.

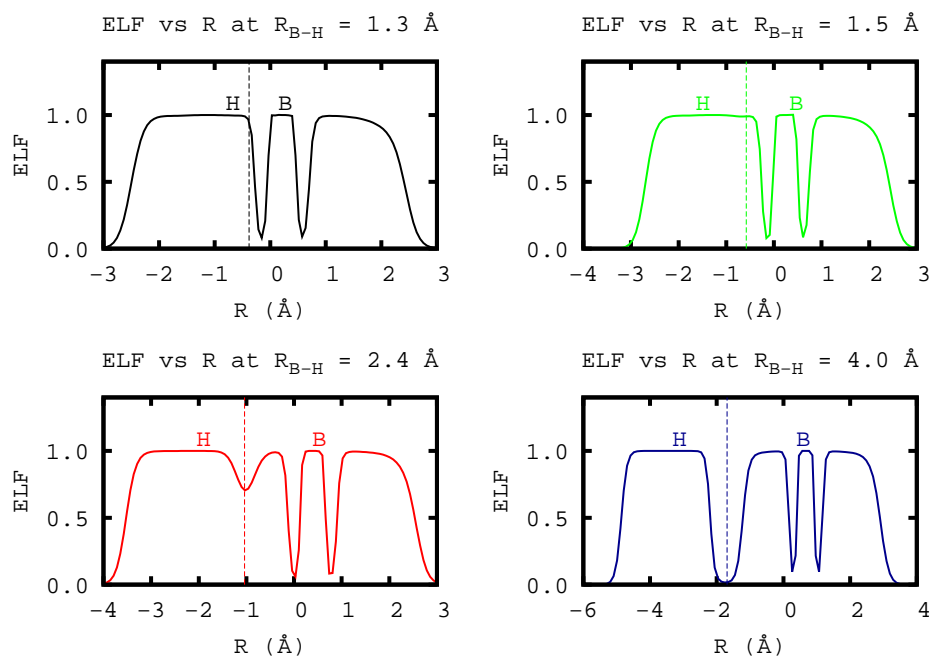

Figure S6: The ELF profile of the  $X^1\Sigma^+$  state of BH along the internuclear axis for several values of the interatomic distance. The zero is located at the center of mass and the vertical dashed line indicates the bond critical point.

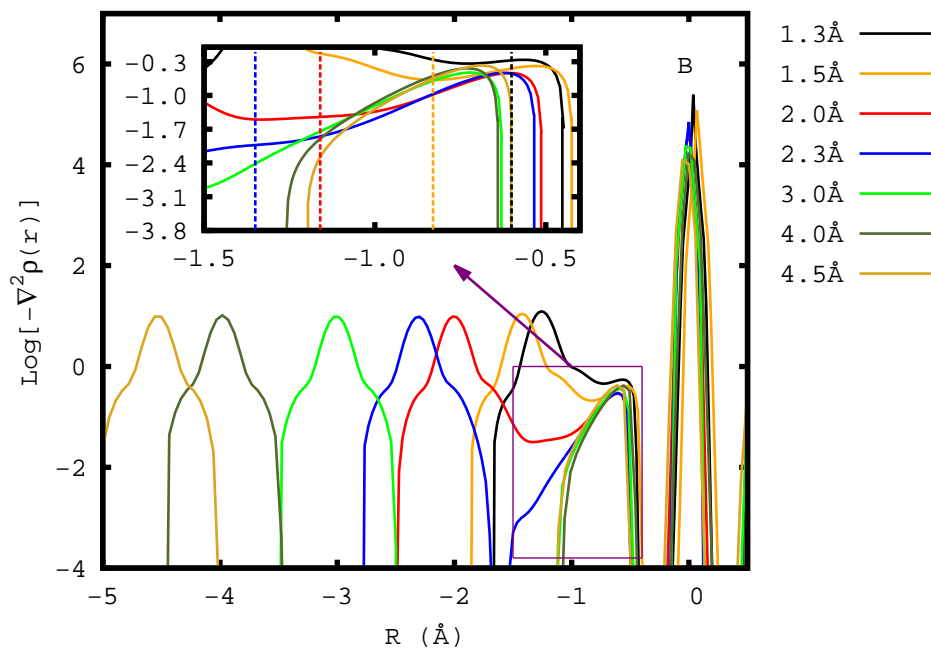

Figure S7: The negative values of the Laplacian of the electron density of BH along the internuclear axis for several interatomic distances. All molecules locate B atom in the z-axis at zero for comparison. The vertical dashed line indicates the bond critical point. Laplacian units are a.u.

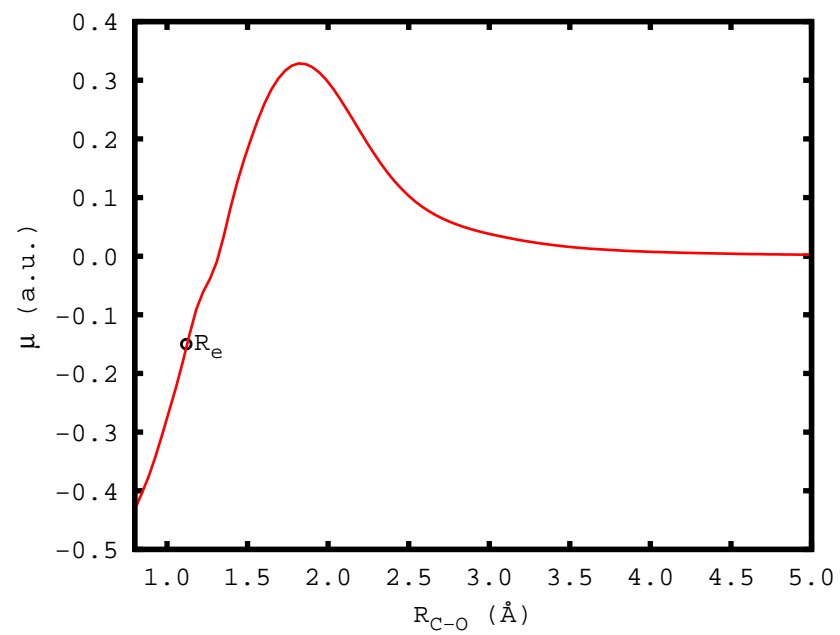

Figure S8: Dipole moment (in a.u.) along the internuclear axis for CO as function of the interatomic distance.



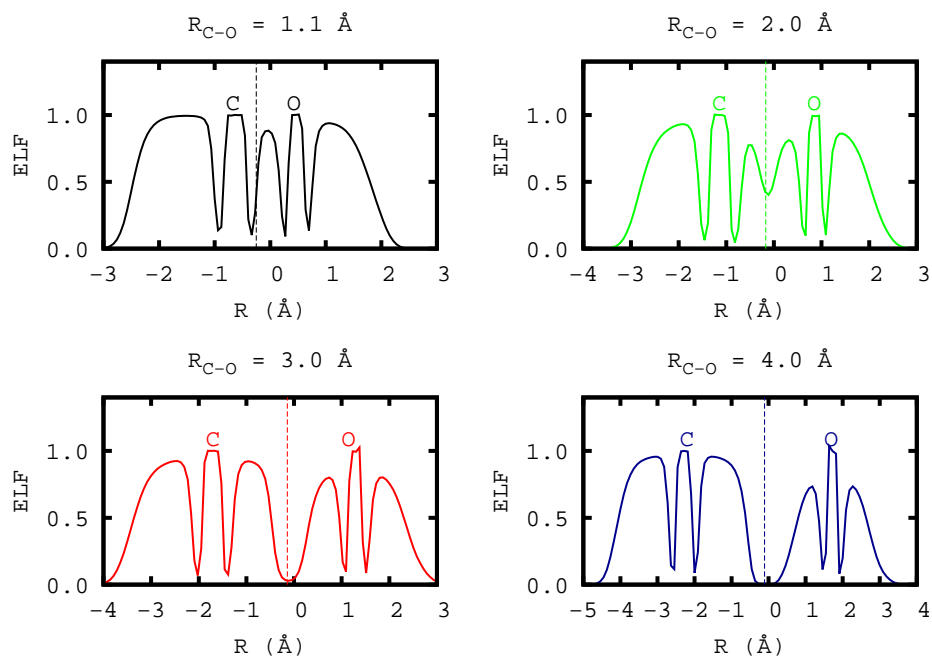

Figure S9: The ELF profile of CO along the internuclear axis for several values of the interatomic distance. The zero is located at the center of mass and the vertical dashed line indicates the bond critical point.

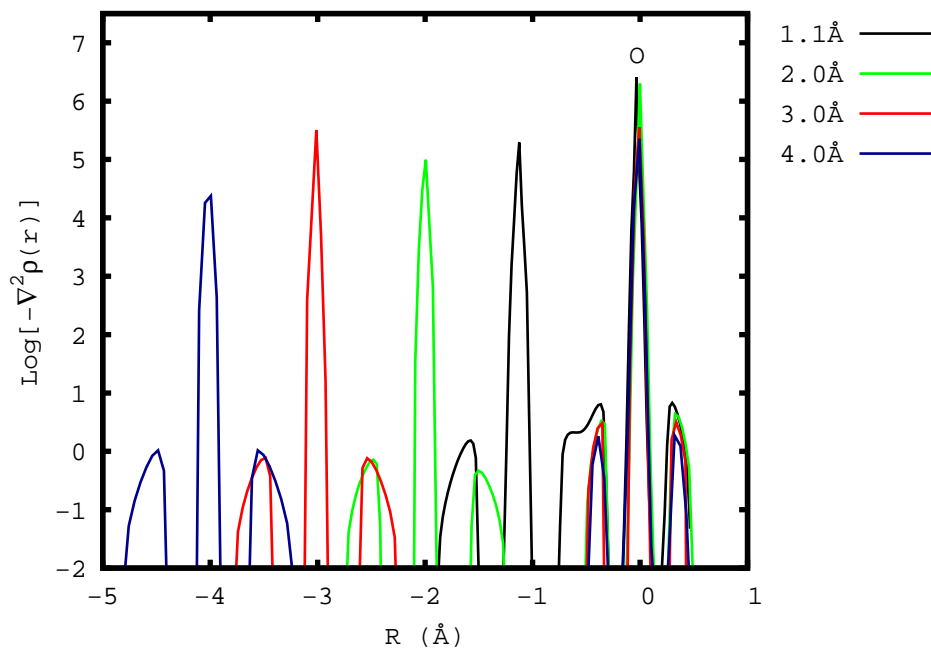

Figure S10: The negative values of the Laplacian of the electron density of CO along the internuclear axis for several interatomic distances. All molecules locate O atom in the z-axis at zero for comparison. The vertical dashed line indicates the bond critical point. Laplacian units are a.u.

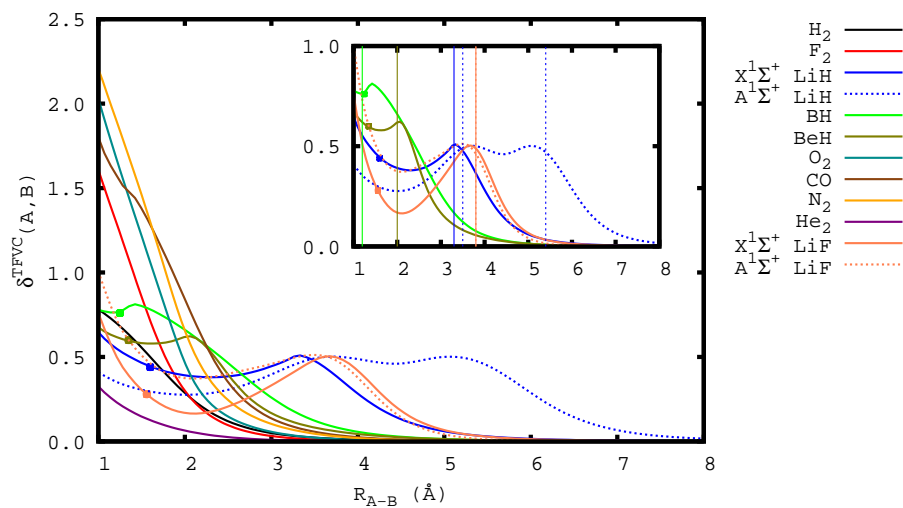

Figure S11: Electron sharing indices calculated using TFVC partition for the series of diatomic molecules. Solid and dotted lines are used for ground states and excited states, respectively. The solid points indicate the position of the equilibrium distance and the vertical lines in the inset plot mark the position of the maximal transfer variation points (see text). ESI units are electron pairs.
